# Supplementary material for: Visual-RFT: Visual Reinforcement Fine-Tuning
Source: arXiv:2503.01785 source file (2025-03-03)
Supplement: Supplementary file 1 [file 6_appendix.tex]

\subsection{Ablation Study}
In our detection experiments, to speed up the evaluation process, we let the model detect the categories present in the image. This testing method is based on the model's ability to effectively determine whether the corresponding objects are present in the image. To validate this approach, we conducted an ablation experiment where, before outputting detection boxes for different objects, the model first checks for the presence of each category. The results, as shown in Tab.~\ref{tab:check_exist_ablation}, indicate that adding a check for object presence leads to a decrease of about 2 points in the overall performance, while the pattern of the experimental results remains unchanged. Therefore, in the detection experiments of the paper, we uniformly adopted the method of detecting the categories present in the image to significantly accelerate the evaluation process and improve testing speed.

\begin{table}[h]
\begin{center}
\caption{
\small
\textbf{Ablation experiment} on object existence judgment.}
\label{tab:check_exist_ablation}
\setlength{\tabcolsep}{4pt}
\scalebox{0.85}
{
\begin{tabular}{ll|l|lllll}
\toprule
\multicolumn{1}{c}{\bf Models} &\multicolumn{1}{c}{\bf Judge} &\multicolumn{1}{c}{\bf $mAP$} &\multicolumn{1}{c}{\bf $AP_{50}$} &\multicolumn{1}{c}{\bf $AP_{75}$} &\multicolumn{1}{c}{\bf $AP_{s}$} &\multicolumn{1}{c}{\bf $AP_{m}$} &\multicolumn{1}{c}{\bf $AP_{l}$}
\\
\midrule
Qwen2-VL-2B & w/o & 9.1 & 16.8 & 8.4 & 1.8 & 9.6 & 17.1\\
Qwen2-VL-2B & w & 6.7 & 12.3 & 6.2 & 1.4 & 7.2 & 12.5\\
% \midrule
% $+$ \methodname & 27.7 & 43.2 & 28.1 & 6.9 & 27.9 & 53.8\\
% $+$ \methodname & 20.7 & 32.5 & 21.1 & 6.4 & 22.7 & 38.2\\
\midrule
Qwen2-VL-7B & w/o & 21.7 & 35.5 & 21.5 & 4.0 & 21.4 & 44.8\\
Qwen2-VL-7B & w & 19.2 & 31.3 & 19.0 & 3.7 & 19.0 & 39.9\\
% \midrule
% $+$ \methodname & 32.0 & 49.9 & 32.6 & 9.8 & 34.2 & 57.9\\
% $+$ \methodname & &  &  &  &  & \\
\bottomrule
\end{tabular}
}
\vspace{-4mm}
\end{center}
\end{table}
